# Supplementary material for: Modular decomposition and analysis of biological networks
Source: arXiv:1412.0742 source file (2014-12-01)

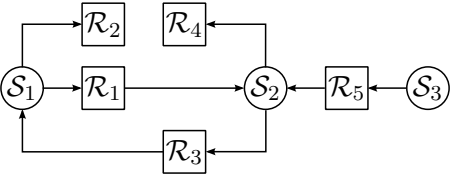

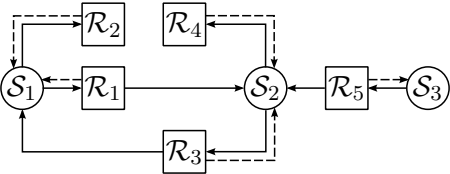

$\mathcal{M}_1$

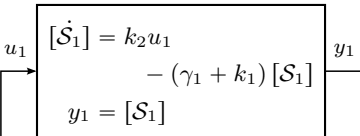

$\mathcal{M}_2$

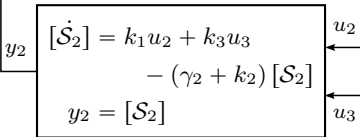

$\mathcal{M}_3$

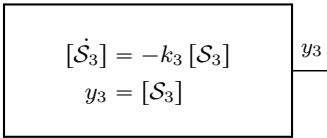

$\mathcal{M}_1$

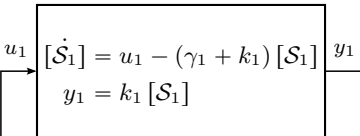

$\mathcal{M}_2$

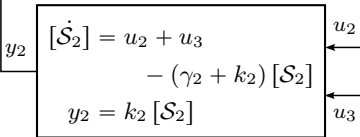

$\mathcal{M}_3$

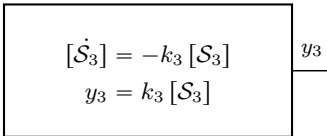

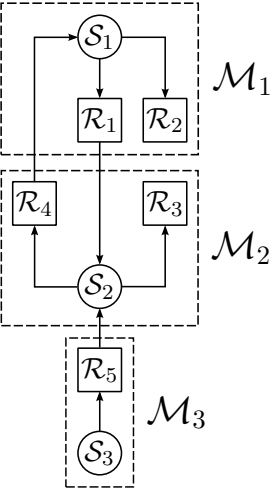

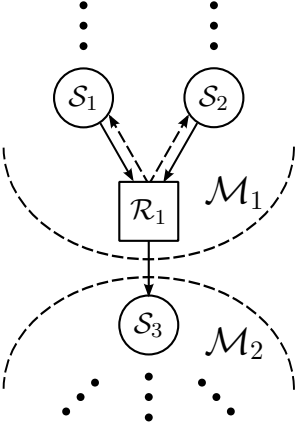

$\mathcal{M}_1$ 

$$[\dot{\mathcal{S}}_1] = -k [\mathcal{S}_1] [\mathcal{S}_2] + \dots$$

$$[\dot{\mathcal{S}}_2] = -k [\mathcal{S}_1] [\mathcal{S}_2] + \dots$$

$$y_1 = k [\mathcal{S}_1] [\mathcal{S}_2]$$

 $u_1$  $y_1$ 

$$[\dot{\mathcal{S}}_3] = u_1 + \dots$$

 $\mathcal{M}_2$

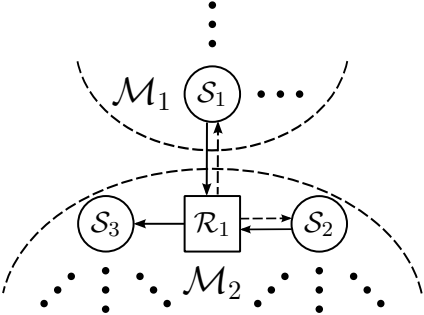



$\mathcal{M}_1$ 

$$[\dot{\mathcal{S}}_1] = -u_1 [\mathcal{S}_1] + \dots$$

$$y_2 = u_1 [\mathcal{S}_1]$$

 $u_1$  $y_1$  $u_2$  $y_2$ 

$$[\dot{\mathcal{S}}_2] = -u_2 + \dots$$

$$[\dot{\mathcal{S}}_3] = u_2 + \dots$$

$$y_1 = k [\mathcal{S}_2]$$

 $\mathcal{M}_2$

$\mathcal{M}_1$ 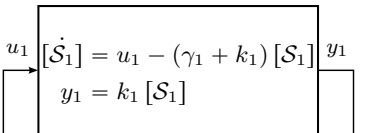 $\mathcal{M}_2$ 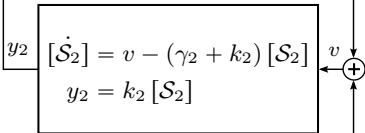 $\mathcal{M}_3$ 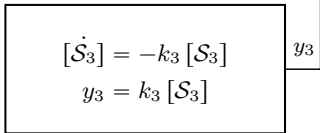

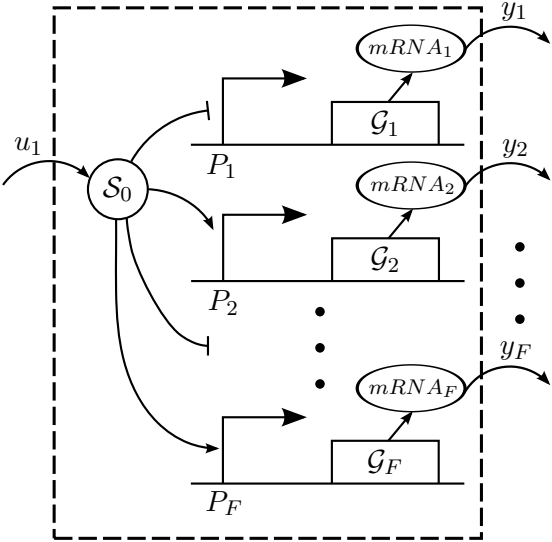

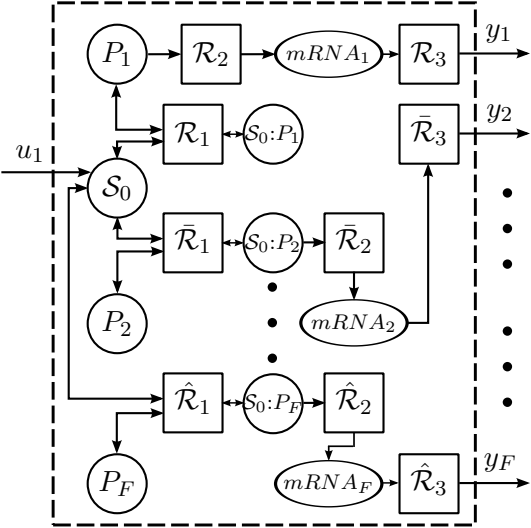

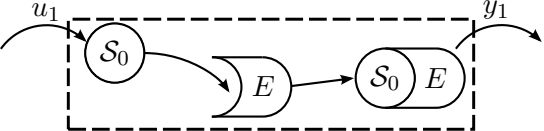

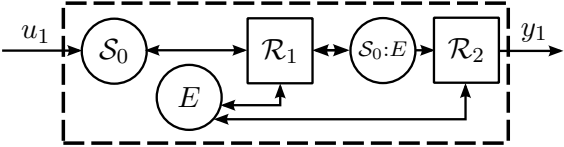

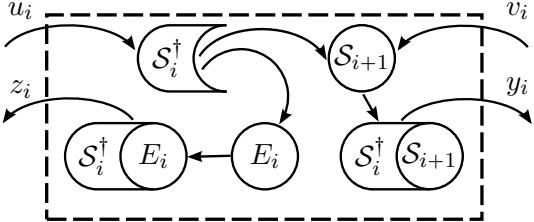

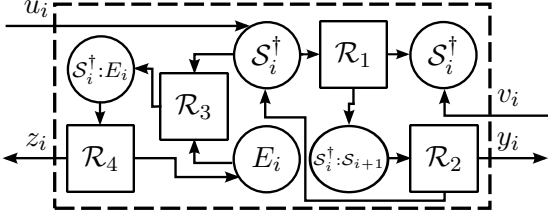



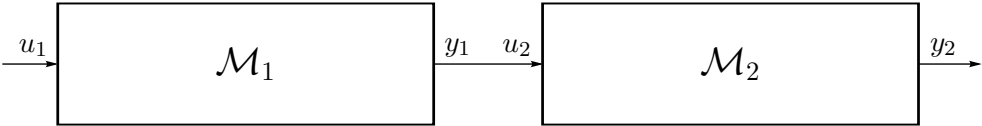

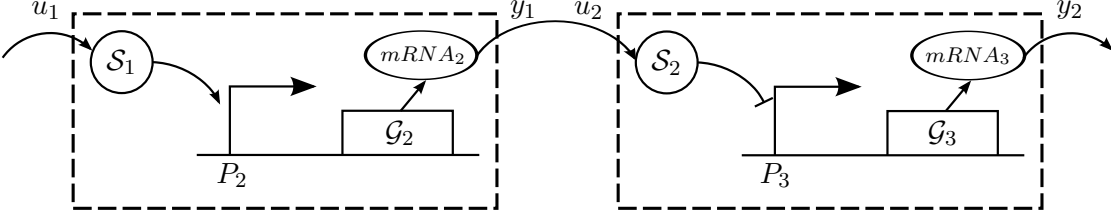

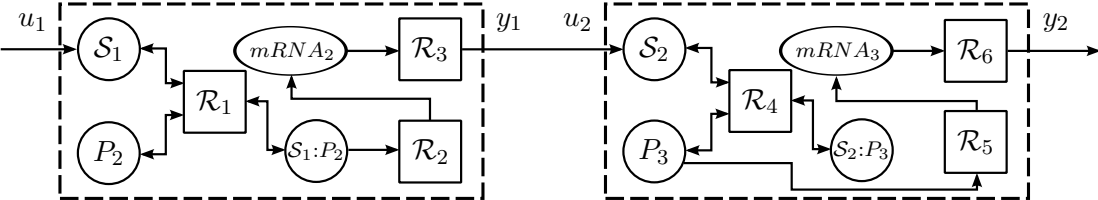

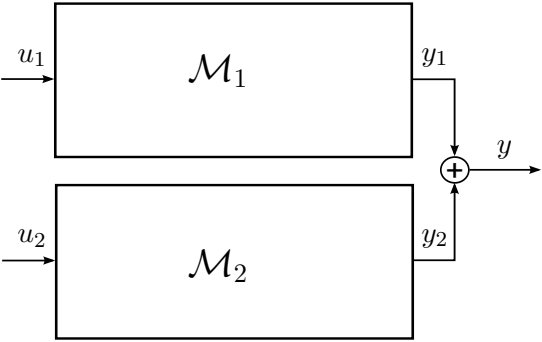

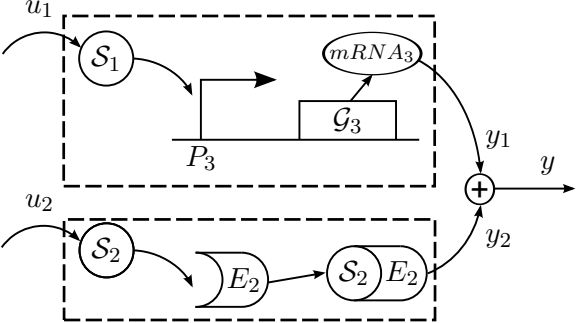

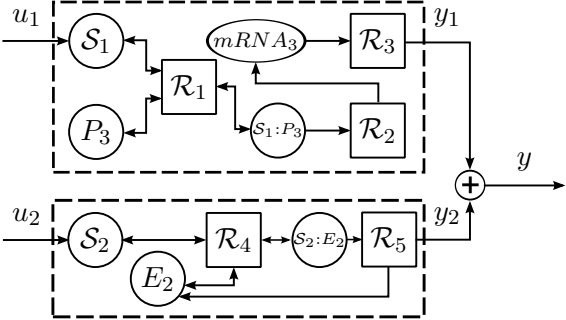

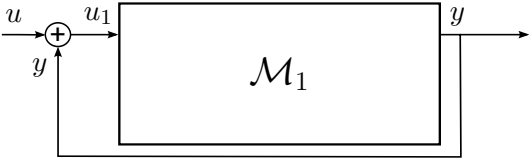

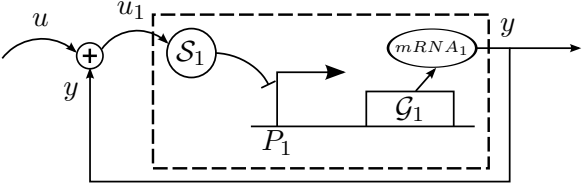



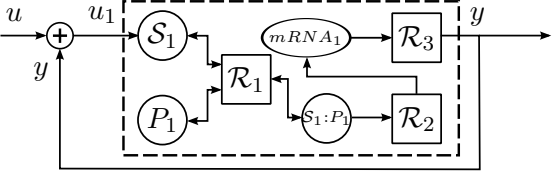

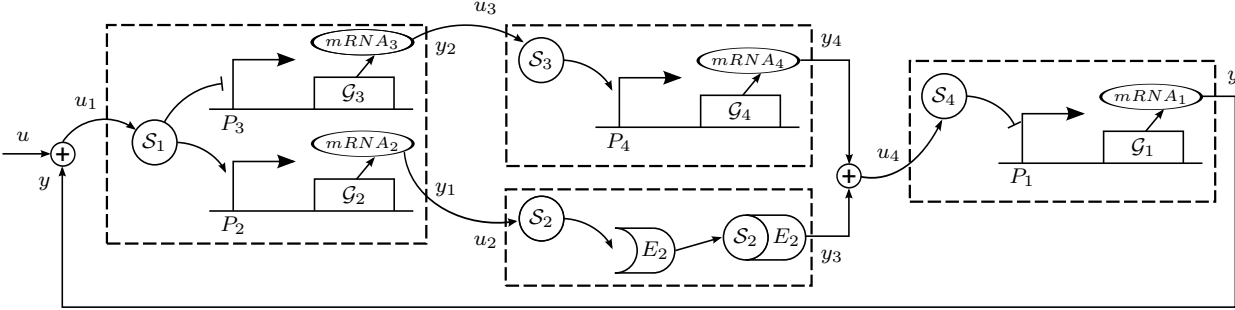

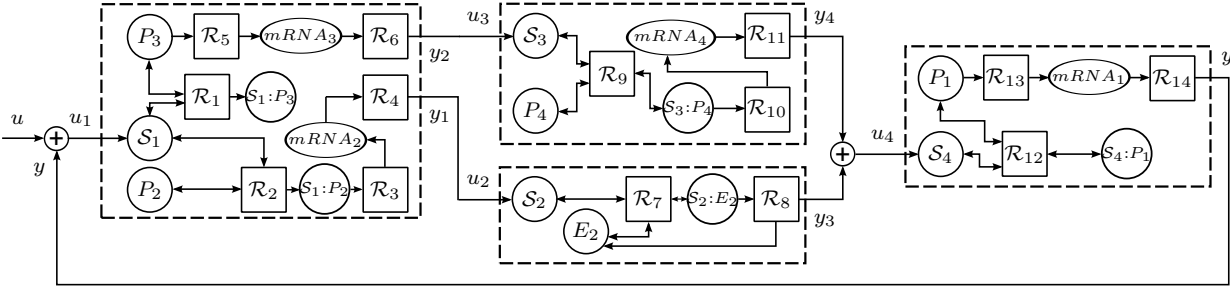

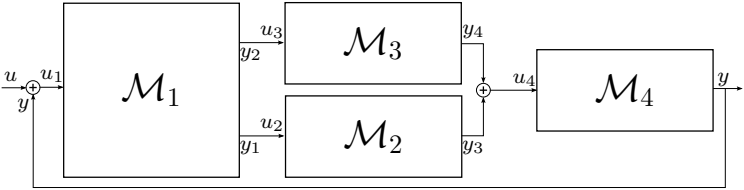

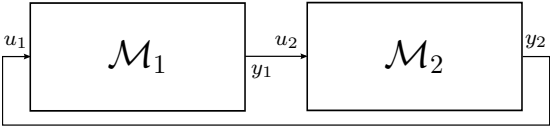

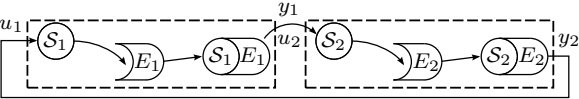

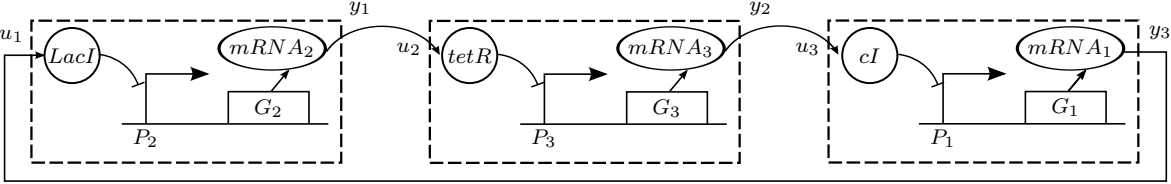

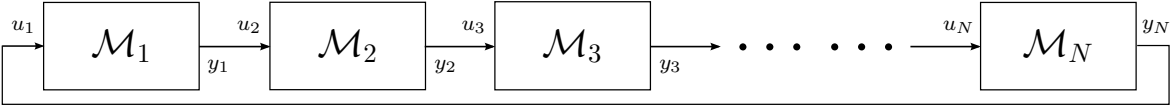



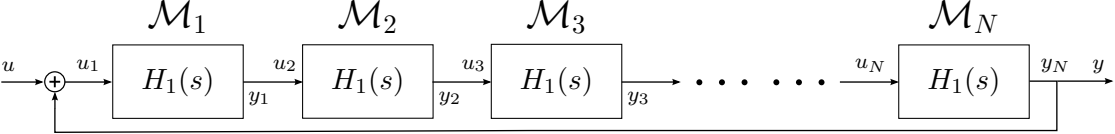

Supplement: Supplementary file 1 [file paper_and_supplemental-pics.pdf]
